# Supplementary material for: The Spike Gating Flow: A Hierarchical Structure Based Spiking Neural Network for Online Gesture Recognition
Source: arXiv:2206.01910 source file (2022-06-07)
Supplement: Supplementary file 1 [file appendixA.tex]

%%%%%%%%% BODY TEXT
\section{Network details}
\label{sec:appendixa}
\subsection{SGF}

\begin{figure}[th]
    \centering
	\includegraphics[width=0.6\columnwidth]{fig/detailed_network.pdf} 
    \caption{The detailed architecture of SGF network.}
    \label{detailed_network}
\end{figure}

The detailed structure of SGF is shown in Fig. \ref{detailed_network}, the red number of output neurons indicate different event types:

\begin{itemize}
\setlength{\itemsep}{0.1ex} 
\item 1: hand clap; 
\item 2: left hand wave;
\item 3: right hand wave;
\item 4: right arm clockwise;
\item 5: right arm counter clockwise;
\item 6: left arm clockwise;
\item 7: left arm counter clockwise;
\item 9: air drum
\item 10: air guitar.
\end{itemize}

At first, SGF unit A classifies actions into four types: 3, 4+5, 6+7 and 1+2+8+9+10. Then SGF unit B detects action types of 4, 5, 6 and 7. Finally, SGF unit C responses for the action 1, 2, 8, 9 and 10.

% SNNs' memory sizes and operation numbers are also displayed in the Tab. \ref{sgf_op_num} and Tab. \ref{sgf_model_size}. Each SNN type has different sub-network numbers, and each individual shares identical functionalities but with different parameters. 

The network parameter calculation is shown in Tab. \ref{sgf_model_size}. Spatial SNNs with feature index A/D, B/C and G have the sub-network number 16, 18 and 2, respectively. And temporal SNNs with feature index E/F and H/I/J/K have the sub-network number 160 and 2. Also, the memory for ST core to store the neuron state is counted as the model size cost, as shown in Tab. \ref{sgf_model_size} first two row. As we can see, the neuron state for ST core takes the largest part of memory consumption, while the feature vector storage is relatively small. Also, Operation number of different networks are displayed in the Tab. \ref{sgf_op_num}. %For example, one element accumulation operation and one element-wise comparison are counted as two operations. The operation number mainly originates from ST core and temporal SNNs, while spatial SNNs only need small operation number.

\begin{table}[t]
    \scriptsize
    \centering
    \begin{tabular}{cccc}  
    \toprule   
    \toprule    
Layer       & Calculation	  & Number   & Model size \\
ST core 1	& 42*42*2*8/8	& 1 & 3528 Byte\\
ST core 2	& 128*128*2*8/8	& 1	& 32768 Byte\\
A/D	        &(110+2*8)/8=19	& 16 & 304 Byte\\
B/C	        &(110+2*8)/8=19	& 18 & 342 Byte\\
G	        &2*8/8	&2	& 4 Byte\\
E/F	        &3*8/8	    &160	&480 Byte\\
H/I/J/K	    &8/8	    &2	&32 Byte\\
\midrule
	    &	    &Total  &36.58KB\\
    \end{tabular}
    \caption{The details of SGF parameter calculation.}
    \label{sgf_model_size}
\end{table}

\begin{table}[t]
    \scriptsize
    \centering
    \begin{tabular}{cccc}  
    \toprule   
    \toprule    
Layer       & Calculation	  & Number   & Operation number \\
ST core 1	& 3*3*42*42*80+42*42*80	& 1 & 1.35 MOPs\\
ST core 2	& 1*1*128*128*80+128*128*80	& 1	& 2.5 MOPs\\
A/D	        & 42*42+(42*42-1)+1	& 16 & 56.0 KOPs\\
B/C	        & 42*42+(42*42-1)+1	& 18 & 63.0 KOPs\\
G	        & 42*42+(42*42-1)+1	& 2	& 7 KOPs\\
E/F	        & (30*30+30)*3*10	& 160	& 4.26 MOPs\\
H/I/J/K	    & (30*30+30)*3*10	& 2	& 54.5 KOPs\\
\midrule
	    &	    &Total  & 8.27 MOPs\\
    \end{tabular}
    \caption{The details of SGF operation number calculation.}
    \label{sgf_op_num}
\end{table}

\newpage
\subsection{ConvNet}

The layer-by-layer computation of parameter and operation number is illustrated in the Table \ref{Convnet} \cite{DBLP:conf/cvpr/AmirTBMMNNAGMKD17}.

\begin{table}[t]
    \scriptsize
    \centering
    \begin{tabular}{cccccccc}  
    \toprule   
    \toprule    
IC	    & OC	    &K	&S	&Pad	&H/W(out)	&Parameters	 &MACs \\
6	    & 12	    &3	&2	&0	    &31	        &648	     &622728\\
12	    & 252	    &4	&2	&0	    &14	        &48384	     &9483264\\
252	    & 256	    &1	&1	&0	    &14	        &64512	     &12644352\\
256	    & 256	    &2	&2	&0	    &7	        &262144	     &12845056\\
256	    & 512	    &3	&1	&1	    &7	        &1179648	 &57802752\\
512	    & 512	    &1	&1	&0	    &7	        &262144	     &12845056\\
512	    & 512	    &1	&1	&0	    &7	        &262144	     &12845056\\
512	    & 512	    &1	&1	&0	    &7	        &262144	     &12845056\\
512	    & 512	    &2	&2	&0	    &3	        &1048576	 &9437184\\
512	    & 1024	    &3	&1	&1	    &3	        &4718592	 &42467328\\
1024	& 1024	    &1	&1	&0	    &3	        &1048576	 &9437184\\
1024	& 1024	    &1	&1	&0	    &3	        &1048576	 &9437184\\
1024	& 1024	    &2	&2	&0	    &1	        &4194304	 &4194304\\
1024	& 1024	    &1	&1	&0	    &1	        &1048576	 &1048576\\
1024	& 968	    &1	&1	&0	    &1	        &991232	     &991232\\
968	    & 2640	    &1	&1	&0	    &1	        &2555520	 &2555520\\
\midrule
        &           &   &   &       & Total     &18995720	 &211501832\\
        &           &   &   &       & Total     &18.12M      &201.70M
    \end{tabular}
    \caption{The process of parameters and MACs of ConvNet.}
    \label{Convnet}
\end{table}

\newpage

\subsection{PAT}

The PAT \cite{DBLP:conf/cvpr/YangZNLLZT19} are formed with 3 sequential GAT and 3 MLP as shown in Table \ref{PAT}.

\begin{table}[t]
    \scriptsize
    \centering
    \begin{tabular}{cccccccc}  
    \toprule   
    \toprule    
Layer type        &N	    & c/IC	    &\#Parameters	 &\#MACs \\
GAT	&1024	&1024	&1024	&349525.3333	&715827882.7\\
GAT	&384	&1024	&1024	&349525.3333	&184549376\\
GAT	&128	&1024	&1024	&349525.3333	&50331648\\
MLP	&64	    &1024	&512	&524288	        &33554432\\
MLP	&64	    &512	&256	&131072	        &8388608\\
MLP	&64	    &256	&10	    &2560	        &163840\\
\midrule
	&		&	    &Total  &1706496	    &992815786.7\\
	&		&	    &Total  &1.63M	        &946.82M\\
    \end{tabular}
    \caption{The process of parameters and MACs of PAT network.}
    \label{PAT}
\end{table}
