# Supplementary material for: The Spike Gating Flow: A Hierarchical Structure Based Spiking Neural Network for Online Gesture Recognition
Source: arXiv:2206.01910 source file (2022-06-07)
Supplement: Supplementary file 2 [file appendixB.tex]

\section{Hardware Implementation}
\label{sec:appendixb}

The appendix \ref{sec:appendixb} presents a conceptual hardware architecture for implementing an SGF inference model (five events classifications).

\subsection{AER Bus}

\begin{figure}[th]
	\centering
	\includegraphics[width=0.45\columnwidth]{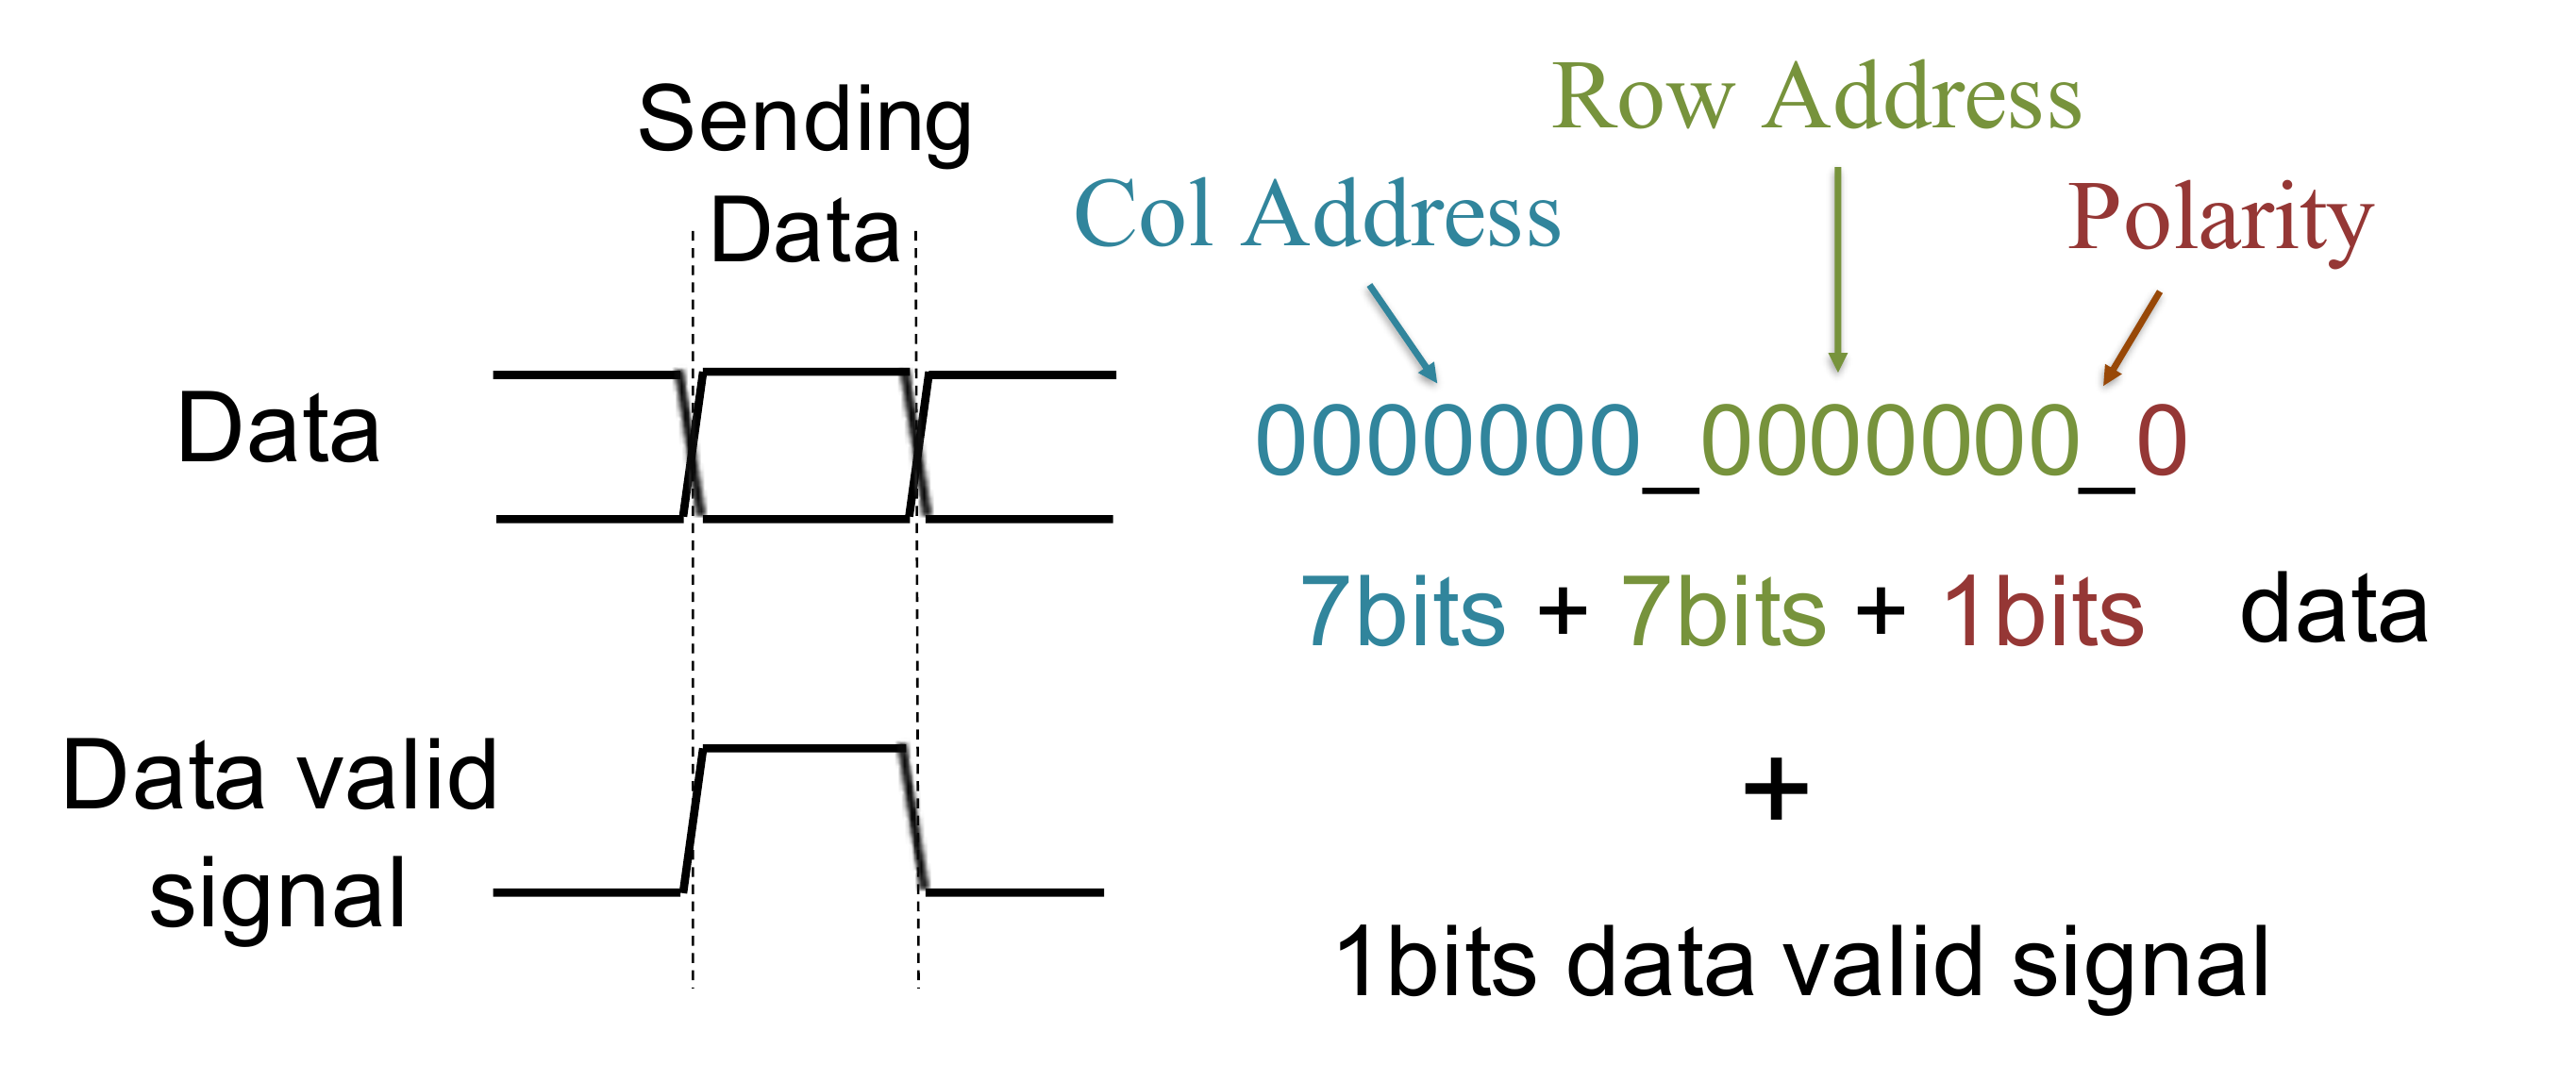} 
	\caption{The timing diagram of AER signals.}
	\label{Fig-aer_timing}
\end{figure}
\begin{figure}[th]
	\centering
	\includegraphics[width=0.3\columnwidth]{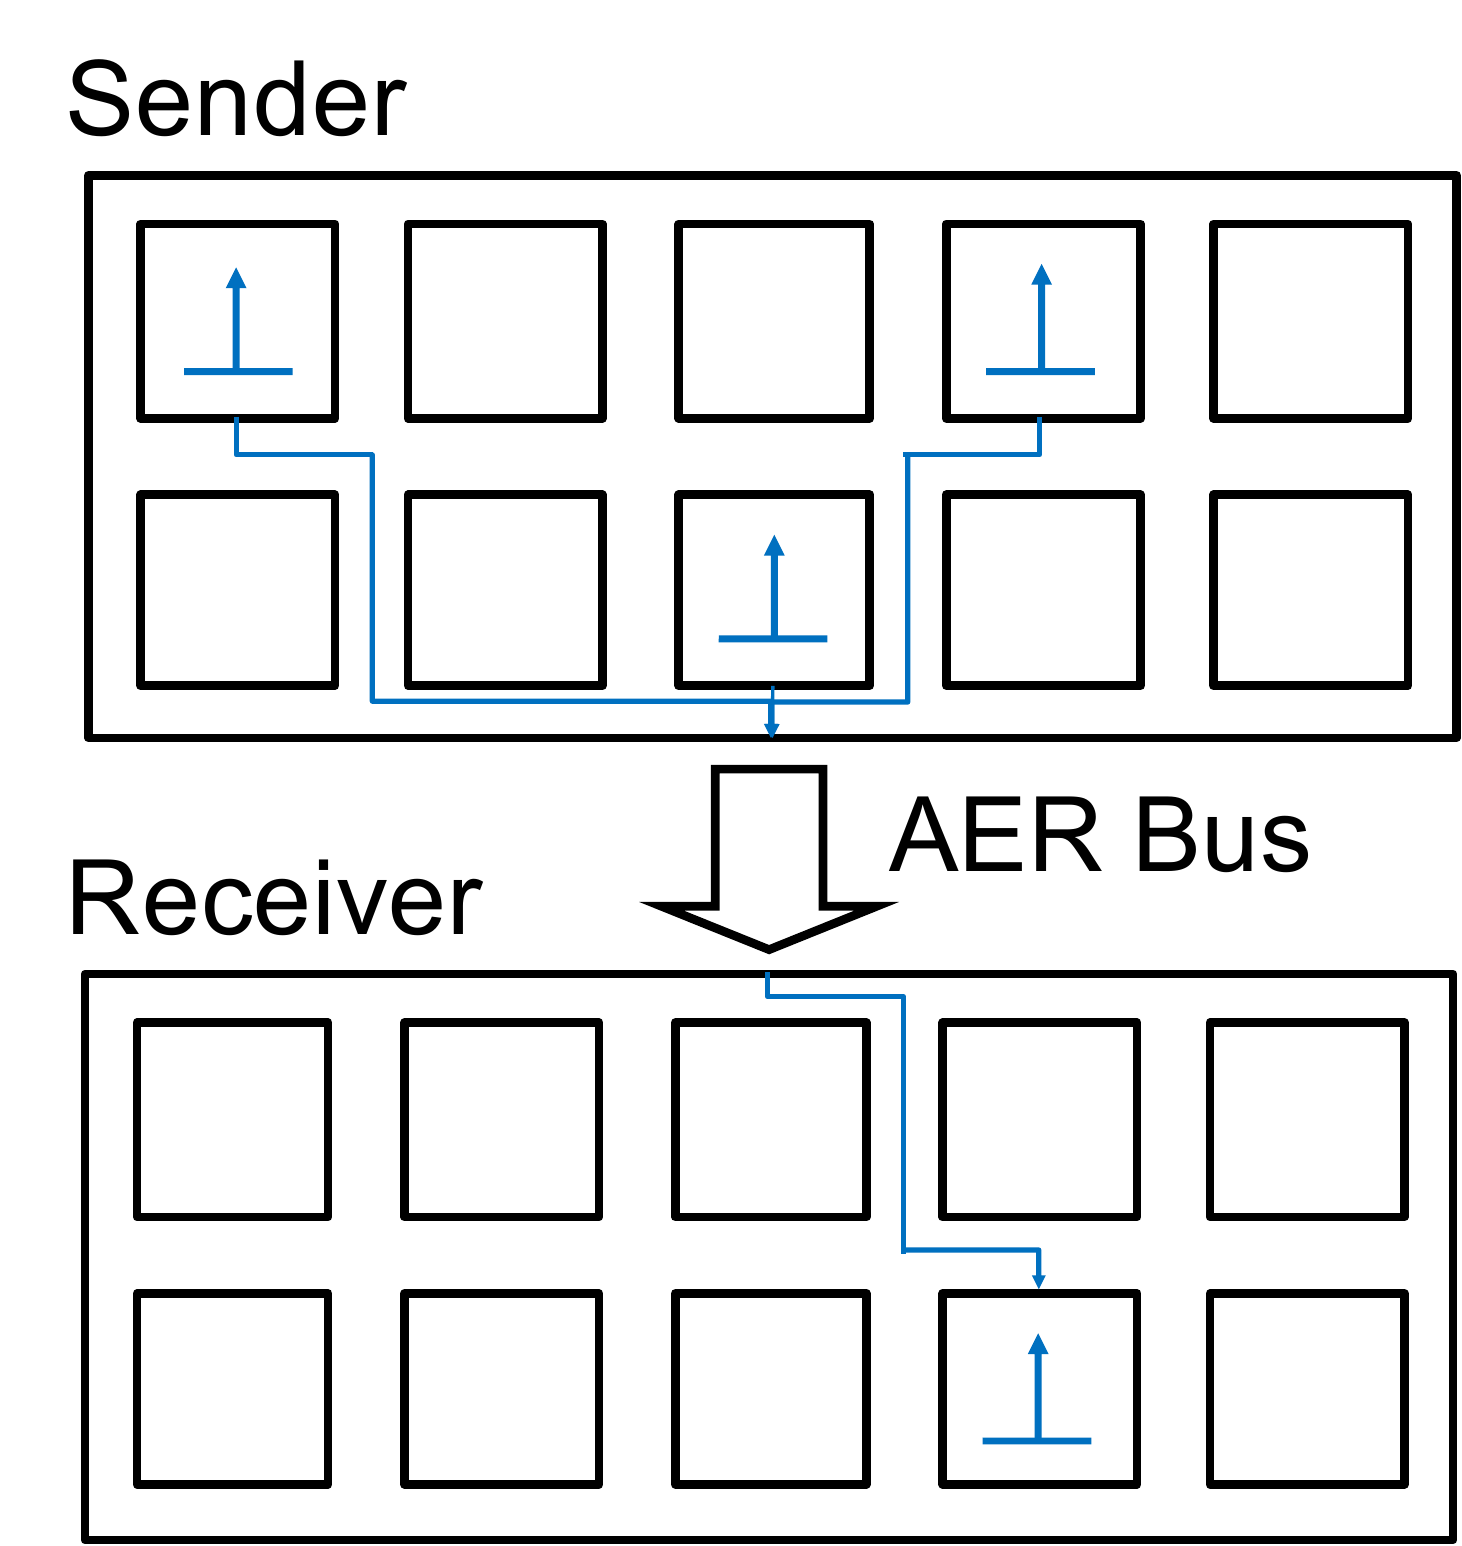} 
	\caption{Schematic diagram of AER communication between modules.}
	\label{Fig-aer}
\end{figure}

In the hardware implementation, the spike based information is transferred among different modules via an Address-Event Representation (AER) communication protocol \cite{aer}. 

As depicted in Fig. \ref{Fig-aer_timing}, the AER data consists of column/row addresses of the source neuron and the polarity of a spike event. In practice, we choose 7-bit for both column and row address, and 1-bit for the polarity. Therefore there are total 15 bits to represent the location and polarity information of a spike. Fig. \ref{Fig-aer} shows how the sender module and the receiver module is communicated by the AER bus. When a spike event is released from an sender module, the output spikes will be packed and push in the AER sending FIFO. In the meantime, the AER bus continuously transmits the data package when the AER sending FIFO is not empty. The destination address is calculated by the receiver module via a look-up table module.

\subsection{Hardware architecture}

An overview of the system is shown in Fig. \ref{Fig-sgf_system}. The system configuration is as below: a PC controller sends configuration commands (e.g. network architecture parameters, threshold parameters) to the FPGA based SGF system, and receives the inference result from the system via a Universal Asynchronous Receiver/Transmitter (UART) protocol. Also, A DVS camera is linked to the SGF system to provide real-time event data. The data paths are labeled as blue lines while the control signals are indicates by the red lines. 

\begin{figure}[th]
	\centering
	\includegraphics[width=0.6\columnwidth]{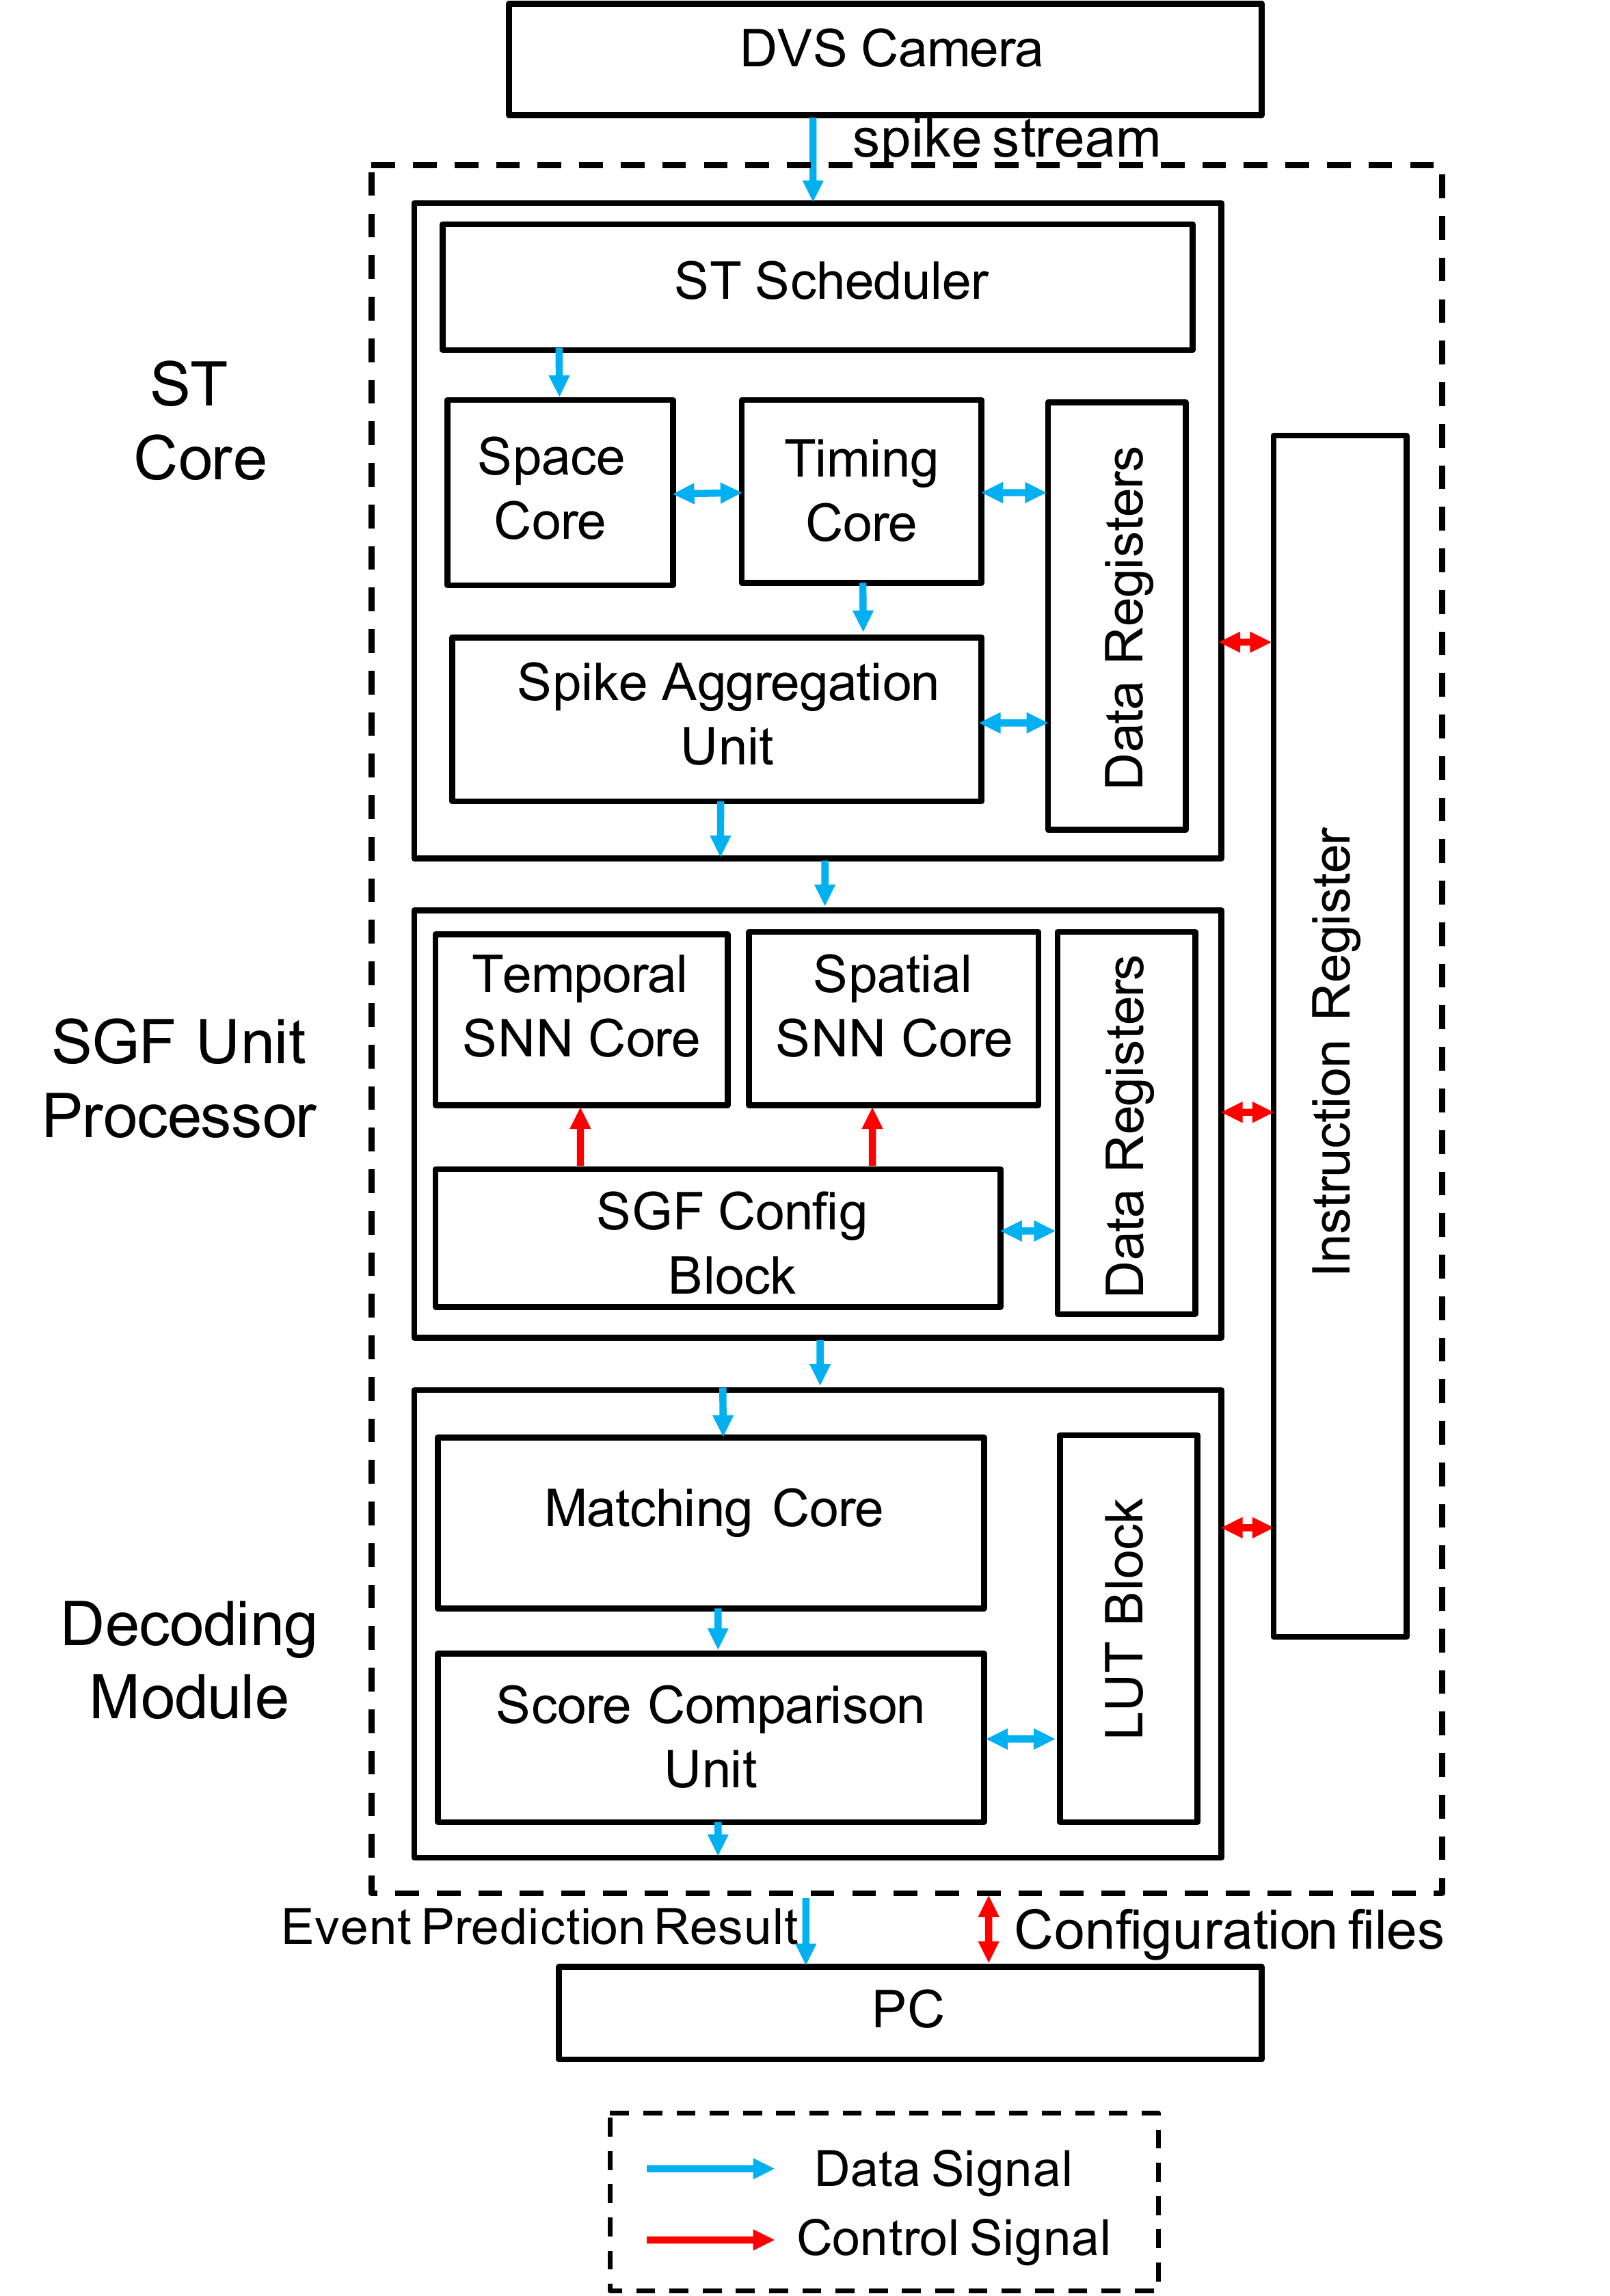} % Reduce the figure size so that it is slightly narrower than the column. Don't use precise values for figure width.This setup will avoid overfull boxes. 
	\caption{An overview of the SGF hardware system.}
	\label{Fig-sgf_system}
\end{figure}

% The sensing layer is to pre-processing the input data. The sensing layer consists of a camera interface, a processing unit and a sensing (SE) memory. It receives the spike input from a Dynamic Vision Sensor (DVS) camera or digital input from a RGB camera. If the input source is a RGB camera, the sensing layer will store the input image and differentiates its pixel value with the next incoming image. If the absolute value of the difference is higher than the pre-setting threshold, the address of this pixel will be recorded in a sending FIFO. If the input source is DVS camera, we just apply Yang’s denoising algorithm to the raw data and obtain the sensing output.

The Spatial-Temporal (ST) core module consists of a Space core (S core) and a Timing core (T core), which response for integrating spikes in the space and time domain. And data registers are employed to save the neurons' status. Also a ST scheduler is implemented to translate the input AER data addresses to the corresponding ST core destination addresses. 

In the SGF unit processor, there are four main components: a temporal SNN cores, a spatial SNN core, a SGF configuration block and data registers. SNN cores can implement several SNNs in a time multiplexing manner. At the initialization stage, a SGF configuration block receives the network architecture information from an instruction register. A SGF network is constructed by combining multiply temporal and spatial SNNs that specifically followed the instructions. The output spikes of SNNs are formed into feature vectors for the next stage processing.

The decoding module is to generate the final inference result. Feature vectors that generated at the training stage are stored in the Look-Up-Table (LUT) block. When the decoding module receives a test feature vector from a SGF unit processor, the matching core will calculate final scores based on the implemented algorithm. After a calculation of all the event types' score, the maximum one will be chosen as the predict result via a score comparison unit.

% The ST response map has the spatial-temporal dynamic of the input video sequence, and the decoding layer is to further process the response map to give the event prediction result. The Decoding layer consists of a LUT-based decoding core. Based on the range and intensity of the different region on the response map, different event types can be classified.
